# Supplementary material for: Constraints Matrix Diffusion based Generative Neural Solver for Vehicle Routing Problems
Source: arXiv:2603.07568 source file (2026-03-08)
Supplement: Supplementary file 1 [file 7appendix.tex]

\begin{algorithm}
\caption{Geometric Augmentation Algorithm}
\label{alg:geometric_augmentation}
\begin{algorithmic}[1]
\REQUIRE CVRP instance\\ $I = (depot, customers, demands, routes)$,
\\symmetry type $symmetry\_type$
\ENSURE Geometrically augmented CVRP instance\\
$I' = (depot', customers', demands, routes)$

\STATE $depot' \gets depot$
\STATE $customers' \gets customers$

\STATE Convert to centered coordinates:\\ $depot_{centered} \gets depot - 0.5$
\STATE $customers_{centered} \gets customers - 0.5$

\STATE Convert to polar coordinates:\\ $(r_{depot}, \theta_{depot}) \gets \text{CartesianToPolar}(depot_{centered})$
\FOR{each customer $c$ in $customers_{centered}$}
    \STATE $(r_c, \theta_c) \gets \text{CartesianToPolar}(c)$
\ENDFOR

\IF{$symmetry\_type = \text{horizontal}$}
    \STATE $\theta_{depot}' \gets -\theta_{depot}$
    \FOR{each customer $c$}
        \STATE $\theta_c' \gets -\theta_c$
    \ENDFOR
\ELSIF{$symmetry\_type = \text{vertical}$}
    \STATE $\theta_{depot}' \gets \pi - \theta_{depot}$
    \FOR{each customer $c$}
        \STATE $\theta_c' \gets \pi - \theta_c$
    \ENDFOR
\ELSIF{$symmetry\_type = \text{diagonal1}$}
    \STATE $\theta_{depot}' \gets \frac{\pi}{2} - \theta_{depot}$
    \FOR{each customer $c$}
        \STATE $\theta_c' \gets \frac{\pi}{2} - \theta_c$
    \ENDFOR
\ELSIF{$symmetry\_type = \text{diagonal2}$}
    \STATE $\theta_{depot}' \gets -\frac{\pi}{2} - \theta_{depot}$
    \FOR{each customer $c$}
        \STATE $\theta_c' \gets -\frac{\pi}{2} - \theta_c$
    \ENDFOR
\ENDIF

\STATE Convert back to Cartesian coordinates:\\ $depot_{transformed} \gets \text{PolarToCartesian}(r_{depot}, \theta_{depot}')$
\FOR{each customer $c$}
    \STATE $c_{transformed} \gets \text{PolarToCartesian}(r_c, \theta_c')$
\ENDFOR

\STATE Restore coordinate system:\\ $depot' \gets depot_{transformed} + 0.5$
\STATE $customers' \gets customers_{transformed} + 0.5$
\STATE Clip coordinates to [0,1]:\\ $depot' \gets \text{Clip}(depot', 0, 1)$
\STATE $customers' \gets \text{Clip}(customers', 0, 1)$

\RETURN $I' = (depot', customers', demands, routes)$

\end{algorithmic}
\end{algorithm}

\begin{algorithm}
\caption{Demand Augmentation Algorithm}
\label{alg:demand_augmentation}
\begin{algorithmic}[1]
\REQUIRE CVRP instance:\\ 
$I = (depot, customers, demands, routes)$\\
augmentation type: $aug\_type$
\ENSURE Demand-augmented CVRP instance\\
$I' = (depot, customers, demands, routes)$

\STATE $demands' \gets demands$

\IF{$aug\_type = \text{reverse}$}
    \FOR{each route $R$ in $routes$}
        \STATE $route\_indices \gets [idx - 1 \text{ for } idx \text{ in } R]$
        \STATE $route\_demands \gets demands[route\_indices]$
        \STATE \\$reversed\_demands\newline \gets \text{Reverse}(route\_demands)$
        \FOR{$i = 0$ to $|route\_indices| - 1$}
            \STATE $demands'[route\_indices[i]] \gets reversed\_demands[i]$
        \ENDFOR
    \ENDFOR
\ELSIF{$aug\_type = \text{shuffle}$}
    \FOR{each route $R$ in $routes$}
        \STATE $route\_indices \gets [idx - 1 \text{ for } idx \text{ in } R]$
        \STATE $route\_demands \gets demands[route\_indices]$
        \STATE $shuffled\_demands \gets \text{Shuffle}(route\_demands)$
        \FOR{$i = 0$ to $|route\_indices| - 1$}
            \STATE $demands'[route\_indices[i]] \gets shuffled\_demands[i]$
        \ENDFOR
    \ENDFOR
\ELSIF{$aug\_type = \text{rotate\_cw}$}
    \FOR{each route $R$ in $routes$}
        \IF{$|R| > 1$}
            \STATE $route\_indices \gets [idx - 1 \text{ for } idx \text{ in } R]$
            \STATE $route\_demands \gets demands[route\_indices]$
            \STATE $shifted\_demands \gets \text{Roll}(route\_demands, 1)$
            \FOR{$i = 0$ to $|route\_indices| - 1$}
                \STATE $demands'[route\_indices[i]] \gets shifted\_demands[i]$
            \ENDFOR
        \ENDIF
    \ENDFOR
\ELSIF{$aug\_type = \text{rotate\_ccw}$}
    \FOR{each route $R$ in $routes$}
        \IF{$|R| > 1$}
            \STATE $route\_indices \gets [idx - 1 \text{ for } idx \text{ in } R]$
            \STATE $route\_demands \gets demands[route\_indices]$
            \STATE $shifted\_demands \gets \text{Roll}(route\_demands, -1)$
            \FOR{$i = 0$ to $|route\_indices| - 1$}
                \STATE $demands'[route\_indices[i]] \gets shifted\_demands[i]$
            \ENDFOR
        \ENDIF
    \ENDFOR
\ENDIF

\RETURN $I' = (depot, customers, demands', routes)$

\end{algorithmic}
\end{algorithm}

% Helper functions
\begin{algorithm}
\caption{Helper Functions}
\label{alg:helper_functions}
\begin{algorithmic}[1]

\STATE \textbf{Function} CartesianToPolar($x, y$)
\STATE $r \gets \sqrt{x^2 + y^2}$
\STATE $\theta \gets \text{atan2}(y, x)$
\RETURN $(r, \theta)$

\STATE \textbf{Function} PolarToCartesian($r, \theta$)
\STATE $x \gets r \cdot \cos(\theta)$
\STATE $y \gets r \cdot \sin(\theta)$
\RETURN $(x, y)$

\STATE \textbf{Function} Clip($value, min, max$)
\RETURN $\max(\min, \min(max, value))$

\STATE \textbf{Function} Reverse($array$)
\RETURN $array[::-1]$

\STATE \textbf{Function} Shuffle($array$)
\STATE $shuffled \gets \text{copy}(array)$
\STATE $\text{random\_shuffle}(shuffled)$
\RETURN $shuffled$

\STATE \textbf{Function} Roll($array, shift$)
\STATE $n \gets |array|$
\STATE $shift \gets shift \bmod n$
\RETURN $array[shift:] + array[:shift]$

\end{algorithmic}
\end{algorithm}
